# Supplementary material for: Quantum Chemistry Simulations of Dominant Products in Lithium-Sulfur Batteries
Source: arXiv:2001.01120 ancillary file (2021-12-30)
Supplement: Supplementary file 1 [file lis_si.pdf]

# Quantum computation of dominant products in lithium-sulfur batteries: Supplementary Information

Julia E. Rice,[1] Tanvi P. Gujarati,[1] Mario Motta,[1] Tyler Y. Takeshita,[2] Eunseok Lee,[2] Joseph A. Latone,[1] and Jeannette M. Garcia[1]

[1)]*IBM Quantum, Almaden Research Center, San Jose, CA 95120, USA*

[2)]*Mercedes Benz Research and Development North America, Sunnyvale, CA 94085, USA*

## DETAILS OF QUANTUM EXPERIMENTS ON QUANTUM HARDWARE.

Hardware experiments used 8192 shots per circuit, and employed readout error mitigation as implemented in Qiskit. To mitigate gate errors, we used a simplified Richardson extrapolation in which two computations are performed: one that uses the original quantum circuit, and another one where each CNOT gate is replaced by 3 CNOT gates. The resulting energies, that we label $E_1$ and $E_3$ respectively, are extrapolated using a linear Ansatz $E_n = E_{ex} + n\Delta E$, leading to

$$E_{ex} = E_1 - \frac{E_3 - E_1}{2} \ . \quad (1)$$

Extrapolated energies are shown in the main text, and intermediate energies in Figure S1.

Statistical uncertainties on energies and dipoles account for shot noise as well as fluctuations in the quantum dynamics of the hardware, and are obtained averaging over 3 independent experiments. This procedure safeguards from underestimate of statistical uncertainties also by yielding statistically uncorrelated samples. Error bars on extrapolated energies are propagates with standard statistical techniques,

$$\sigma_{E_{ex}} = \sqrt{\left(\frac{3\,\sigma_{E_1}}{2}\right)^2 + \left(\frac{\sigma_{E_2}}{2}\right)^2} \ . \quad (2)$$

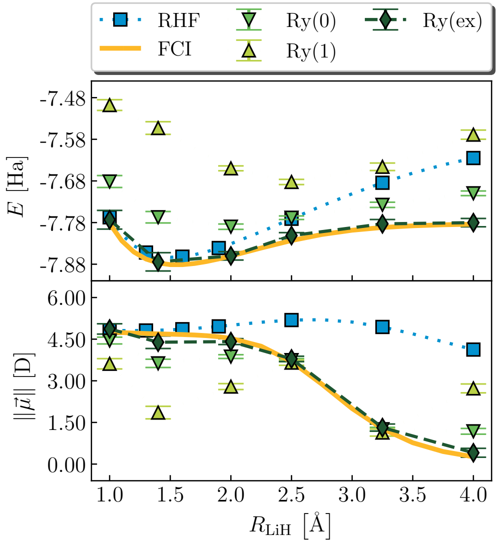


Figure S 1: Ground-state potential energy surface and dipole moment (top, bottom) for LiH from VQE (light-green down-pointing and green up-pointing triangles for points 0 and 1 of the Richardson extrapolation, dark-green diamonds for extrapolated results) and FCI (solid line).

## DETAILS OF CLASSICAL CHEMISTRY SIMULATIONS

In this Subsection, we provide additional details about the chemical species studied in this work. In Table SI, we list the molecular geometries studied in this work. For LiH and $H_2S$, the equilibrium geometries were obtained from the CCCBDB database[1]. For $Li_2S$, we performed an MP2/aug-cc-pV(D+d)Z geometry optimization. For LiSH, we obtained the equilibrium geometry from the textbook Ref [2].

| species | equilibrium values | symmetry | $2n$ | $m$ | frozen orbitals |
|---|---|---|---|---|---|
| LiH | $R_{\rm LiH} = 1.595$ Å | $C_{\infty v}$ | 6 | 4 | Li(1s,2p$_x$,2p$_y$) |
| $H_2S$ | $R_{\rm SH} = 1.3356$ Å<br>$\theta_{\rm HSH} = 92.11°$ | $C_{2v}$ | 12 | 9 | S(1s,2s,2p) |
| $Li_2S$ | $R_{\rm LiS} = 2.1053$ Å<br>$\theta_{\rm LiSLi} = 134.86°$ | $C_{2v}$ | 24 | 21 | Li(1s)<br>Li(1s)<br>S(1s,2s,2p) |
| LiSH | $R_{\rm LiS} = 2.146$ Å<br>$R_{\rm SH} = 1.353$ Å<br>$\theta_{\rm LiSH} = 93.00°$ | $C_s$ | 18 | 15 | Li(1s)<br>S(1s,2s,2p) |

TABLE SI: List of the chemical species investigated in the present work. For each species, we list the investigated geometries, specified in terms of internal coordinates. Whenever internal coordinates are fixed at chosen values, the latter correspond with the quantities listed in column 3. For each species we show the frozen orbitals, molecular symmetry group and number of spin-orbitals ($2n$) and qubits ($m$). $R$ denotes a free parameter, that we vary between 0.5 and 6.0 Å depending on the species of interest.

## ADDITIONAL ELECTRONIC STRUCTURE SIMULATIONS

Due to the current limitations of simulators and hardware, in the present work we focused on minimal basis sets. In order to further establish the physical observations of our work on a more robust ground, in this section we reconsider the species studied in the main text and study their electronic structure using Pople[3] (6-31G, 6-31++G**) and Dunning[4] (cc-pVxZ with

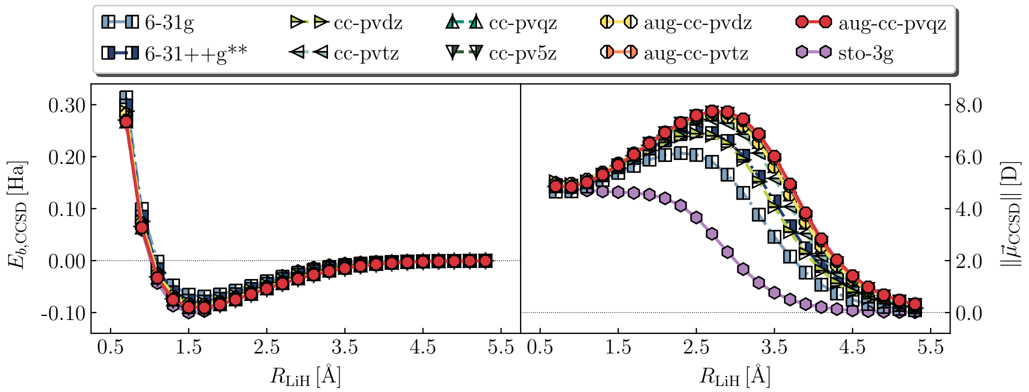


Figure S2: CCSD binding energy (left) and dipole moment (right) for LiH, using various basis sets.

x=D,T,Q,5 and aug-cc-pVxZ with x=D,T,Q) basis sets. We use the CCSD method which, as seen in the main text, has accuracy comparable with the q-UCCSD method. In Figure S2, we consider the dissociation of LiH molecule. For each basis, we show the CCSD binding energies

$$E_{b,\mathrm{CCSD}}(R) = E_{\mathrm{CCSD}}(\mathrm{LiH}, R) - E_{\mathrm{CCSD}}(\mathrm{Li}) - E_{\mathrm{CCSD}}(\mathrm{H}) \;, \quad (3)$$

and norm of the dipole moment, $\|\vec{\mu}_m\|(R)$. As seen, the STO-3G basis provides a qualitatively correct description of the binding energy and dipole moment along dissociation.

## REFERENCES

[1] R. D. Johnson III, "NIST Computational Chemistry Comparison and Benchmark Database, NIST Standard Reference Database Number 101," Tech. Rep. (NIST, 2020).

[2] E. Hirota, K. Kuchitsu, W. J. Lafferty, and D. Ramsey, *Structure data of free polyatomic molecules* (Springer, 1995).

[3] R. Ditchfield, W. J. Hehre, and J. A. Pople, "Self-consistent molecular-orbital methods.IX. An extended Gaussian-type basis for molecular-orbital studies of organic molecules," J. Chem. Phys **54**, 724–728 (1971).

[4] T. H. Dunning Jr, "Gaussian basis sets for use in correlated molecular calculations. I. The atoms boron through neon and hydrogen," J. Chem. Phys **90**, 1007–1023 (1989).
